# Supplementary material for: Interactive Power to Frequency Dynamics Between Grid-Forming Inverters and Synchronous Generators in Power Electronics-Dominated Power Systems
Source: arXiv:2102.12332 source file (2022-10-08)
Supplement: Supplementary file 1 [file appendix.tex]

{\footnotesize
\section*{Appendix}
\label{sec:appendix}
% \subsection{Grid-Forming Inverter}
% The per unit parameters of the generic GFM inverter used in these PSCAD simulations are provided in Table \ref{tab: GFM default parameters}.

\begin{table}[htbp]
    \scriptsize
    \centering
    \caption{GFM parameters; all in per unit.}
    
    \begin{tabular}{c|c||c|c||c|c}
    \textbf{Parameter} & \textbf{Value} & \textbf{Par...} & \textbf{Value} & \textbf{Par...} & \textbf{Value}\\\hline\hline
    $L_f$ & 0.15 & $R_f$ & 0.005 & $C_f$ & 2.5\\\hline
    $R_{cap}$ & 0.005 & $L_c$ & 0.15 & $R_c$ & 0.005\\\hline $k_C^i$ & 1.19 & $k_C^p$ & 0.73 & $G_C$ & 1.0\\\hline
    $k_V^i$ & 1.16 & $k_V^p$ & 0.52 & $G_V$ & 1.0\\\hline
    $k_{V,DC}^i$ & 9179 & $k_{V,DC}^p$ & 73.0 & $k_{i,DC}^i$ & 23031\\\hline
    $k_{i,DC}^p$ & 18.3 & $\Delta V$ & 10\% & $C_{DC}$ & 1 cycle\\\hline
    $L_{DC}$ & 0.000795 & -- & -- & -- & --

    \end{tabular}
    \label{tab: GFM default parameters}
\end{table}

% \subsection{Synchronous Generator}
% The parameters of the SG used in these PSCAD simulations are provided in Table \ref{tab:SG parameters}, where all are in per unit unless units are provided.

\begin{table}[htbp]
    \scriptsize
    \centering
    \caption{SG parameters; per unit unless noted.}
    
    \begin{tabular}{c|c||c|c||c|c}
    \textbf{Parameter} & \textbf{Value} & \textbf{Par...} & \textbf{Value} & \textbf{Par...} & \textbf{Value}\\\hline\hline
    $T_G$ & 0.5 s & $R_{Windage}$ & 0.01 & $H$ & 6 s\\\hline
    $X_d$ & 0.92 & $X_d^{'}$ & 0.169 & $T_{do}^{'}$ & 4.3 s\\\hline
    $X_d^{''}$ & 0.135 & $T_{do}^{''}$ & 0.032 s & $X_q$ & 0.51\\\hline
    $X_{q}^{'}$ & 0.228 & $T_{qo}^{'}$ & 0.85 s & $X_{q}^{''}$ & 0.2\\\hline
    $T_{qo}^{''}$ & 0.05 s & $K_{P,R}$ & 12.77 & $K_{I,R}$ & 20 \\\hline
    $K_{P,A}$ & 20 & $K_{I,A}$ & 1 & $T_E$ & 1.945 s
    \end{tabular}
    \label{tab:SG parameters}
\end{table}

}
